# Supplementary material for: Springer Motives
Source: arXiv:1812.04796 source file (2020-08-04)
Supplement: Supplementary file 1 [file appendix.tex]

%!TEX root = ../main.tex
